# Supplementary material for: Climatology of severe local storm environments and synoptic-scale features over North America in ERA5 reanalysis and CAM6 simulation
Source: arXiv:2005.05489 ancillary file (2020-05-11)
Supplement: Supplementary file 1 [file supplementary.pdf]

# Supplementary Information: Climatology of severe local storm environments and large-scale features over North America in ERA5 reanalysis and CAM6 simulation

*

# LIST OF FIGURES

**Fig. S1.** The number (magenta text) and number percentage (%; filled circles) of radiosonde observations for the period 1998–2014 (twice daily at 0000 and 1200 UTC) at each station, given (a) quality control, (b) quality control and CAPE $\geq$ 0 J kg$^{-1}$, and (c) quality control and CAPE $\geq$ 500 J kg$^{-1}$. . . . . . . . . . . . . . . . . . . . . . . . 3

**Fig. S2.** As in Fig. 3, but the evaluation of CAPE (and thus CAPES06 and EHI03) is for cases with CAPE $\geq$ 0 J kg$^{-1}$ from radiosondes (sample size: supplementary Fig. S1b). . . . . . . . 4

**Fig. S3.** As in Fig. 4, but for the difference (CAM6 minus ERA5). . . . . . . . . . . . . . 5

**Fig. S4.** As in Fig. 4, but for (a) 95th, (b) 90th, and (c) 75th percentiles of CAPES06, EHI03, CAPE, S06, and SRH03 in ERA5 and CAM6. . . . . . . . . . . . . . . . . . . . . 6

**Fig. S5.** As in Fig. 4, but for the 99th percentile of CIN (defined as the negative integral of buoyancy from surface to the level of free convection) from (a) ERA5 and (b) CAM6. . . . . . . . 7

**Fig. S6.** As in Fig. 5–6, but for the difference (CAM6 minus ERA5). . . . . . . . . . . . . 8

**Fig. S7.** Mean number of days associated with severe weather environments (NDSEV) from ERA5 reanalysis data during 1980–2014. For CAPES06 $\geq 10^4$ m$^3$ s$^{-3}$: (a) annually, (b) winter (DJF), (c) spring (MAM), (d) summer (JJA), and (e) fall (SON). (f-j) as in (a-e) but for CAPES06 $\geq 2\times10^4$ m$^3$ s$^{-3}$. (k-o) as in (a-e) but for EHI03 $\geq$ 1. Grey contour lines denote elevations at 500, 1500, and 2500 m. . . . . . . . . . . . . . . . . . . . . 9

**Fig. S8.** As in Fig. 7–8, but for the difference (CAM6 minus ERA5). . . . . . . . . . . . . 10

**Fig. S9.** ERA5 reanalysis vs. CAM6 simulation for the annual and seasonal mean state of atmosphere during 1980–2014. (a) for 10-m wind vector, 2-m air temperature (°C; black contour lines), and 2-m specific humidity (g kg$^{-1}$; filled contours); (b) for 700-hPa wind vector, air temperature (°C; black contour lines), and specific humidity (g kg$^{-1}$; filled contours); (c) for 250-hPa wind vector, geopotential height (m; black contour lines), and wind speed (kts; filled contours). . . . . . . . . . . . . . . . . . . . . . . . . 11

**Fig. S10.** As in Fig. 15, but for sub-regions of (a) R2, (b) R3, (c) R4, and (d) R5. . . . . . . . . 12

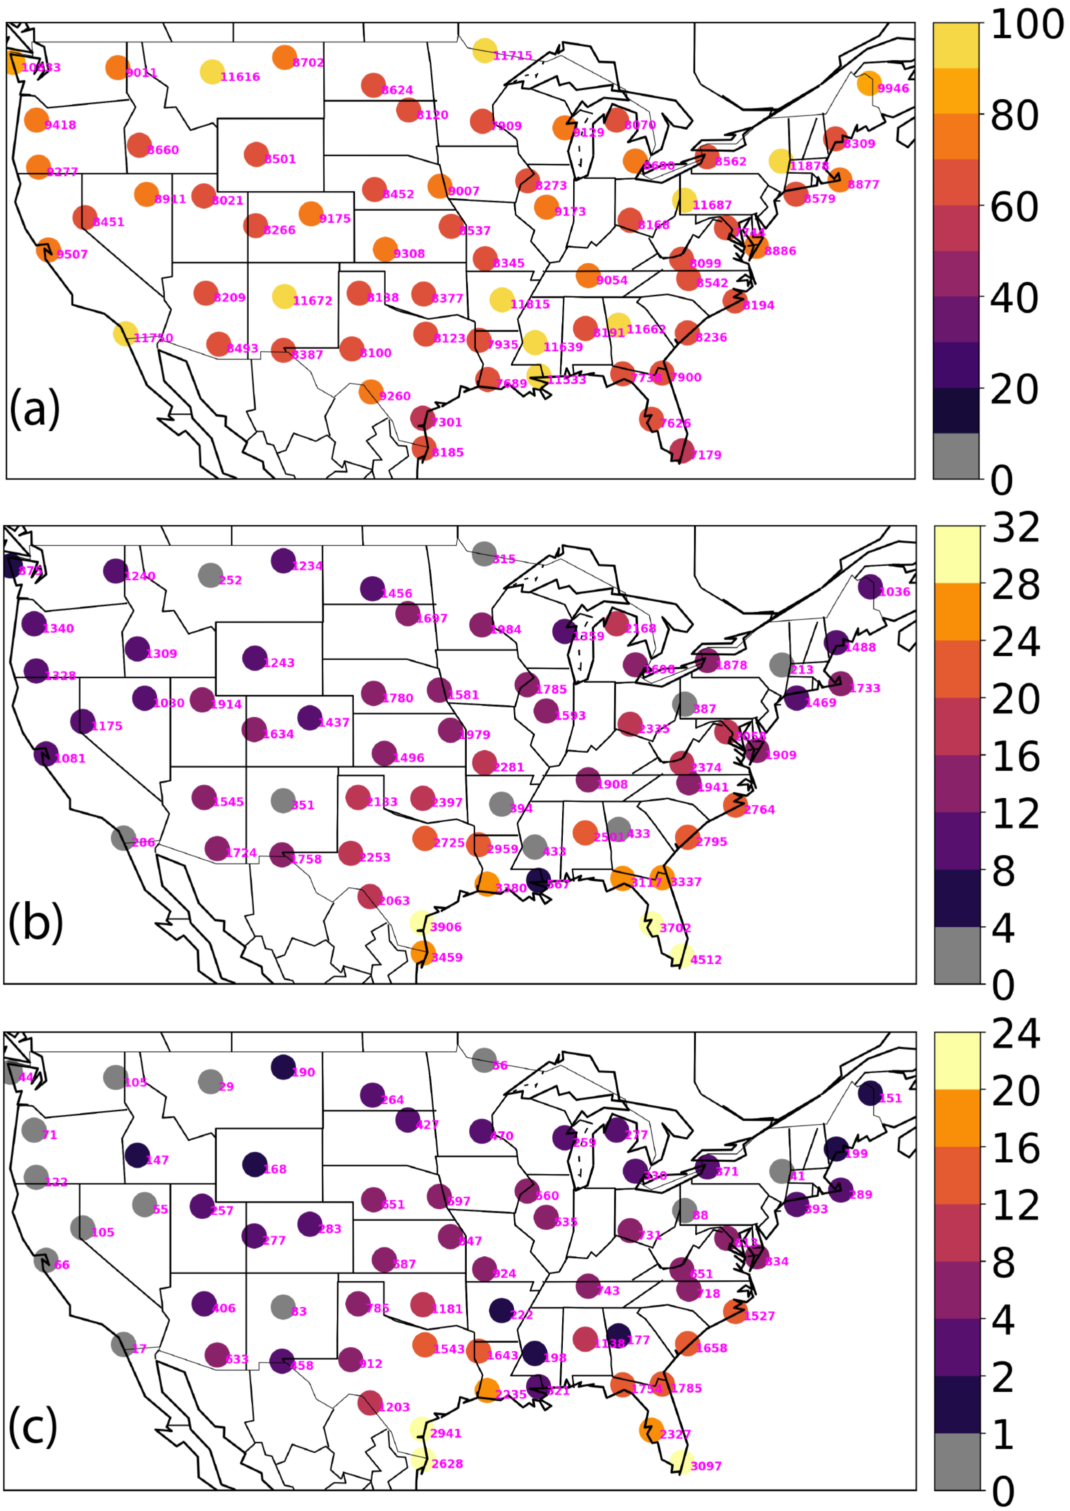


FIG. S1: The number (magenta text) and number percentage (%; filled circles) of radiosonde observations for the period 1998–2014 (twice daily at 0000 and 1200 UTC) at each station, given (a) quality control, (b) quality control and CAPE $\geq$ 0 J kg$^{-1}$, and (c) quality control and CAPE $\geq$ 500 J kg$^{-1}$.

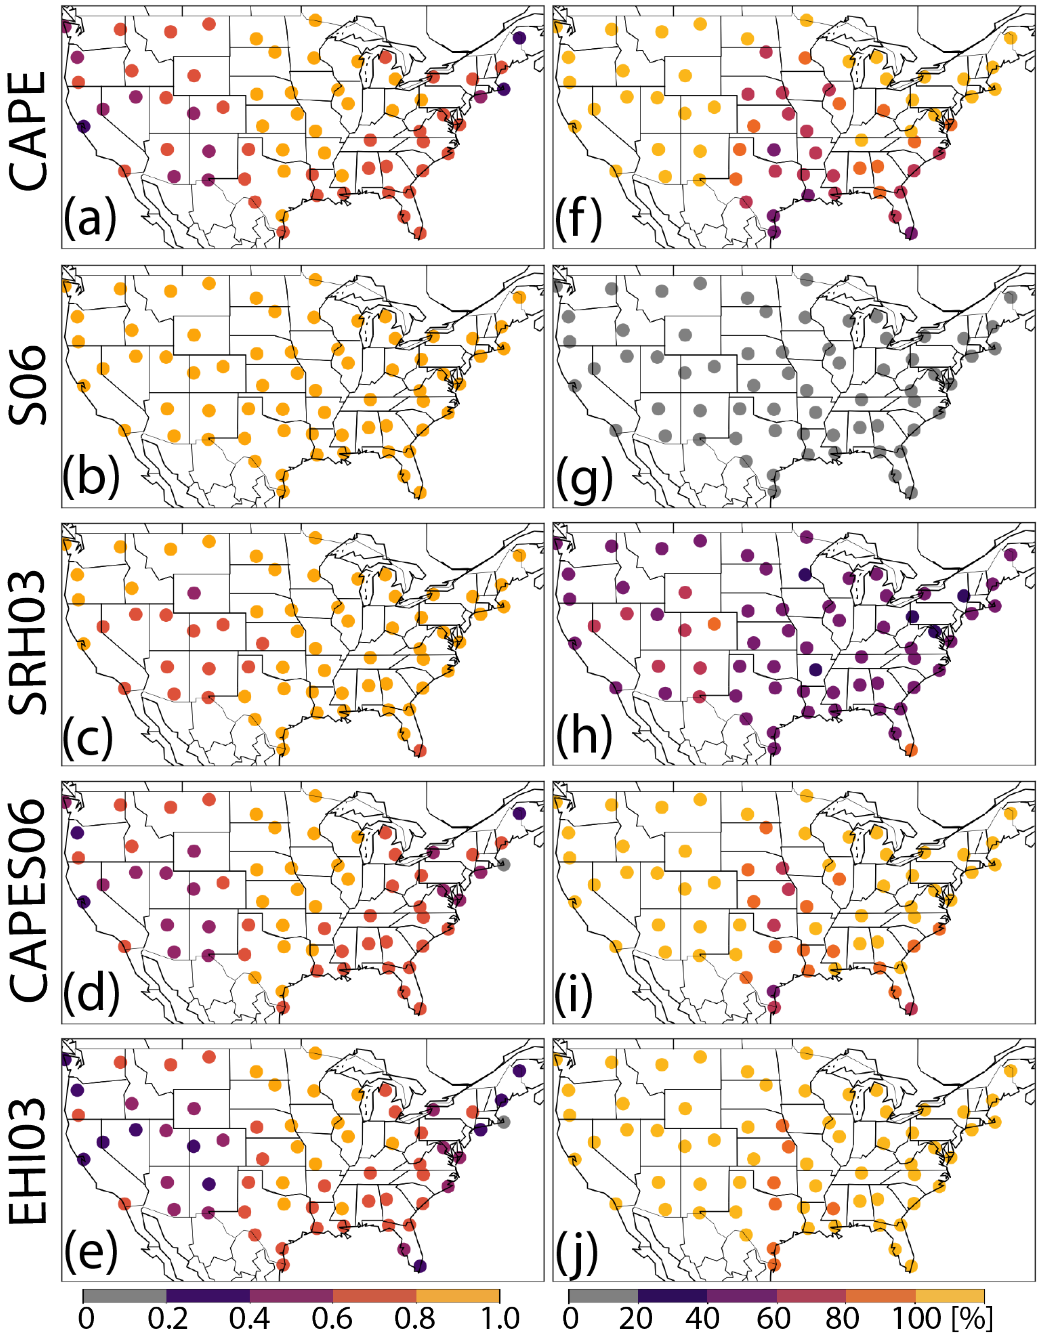


FIG. S2: As in Fig. 3, but the evaluation of CAPE (and thus CAPES06 and EHI03) is for cases with CAPE $\geq 0$ J kg$^{-1}$ from radiosondes (sample size: supplementary Fig. S1b).

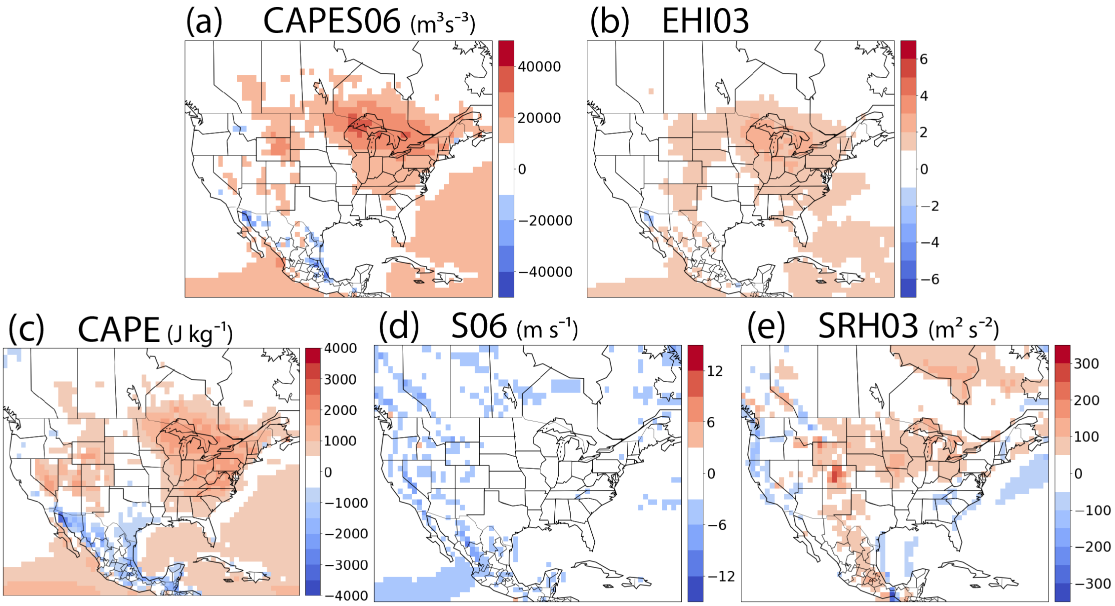


FIG. S3: As in Fig. 4, but for the difference (CAM6 minus ERA5).

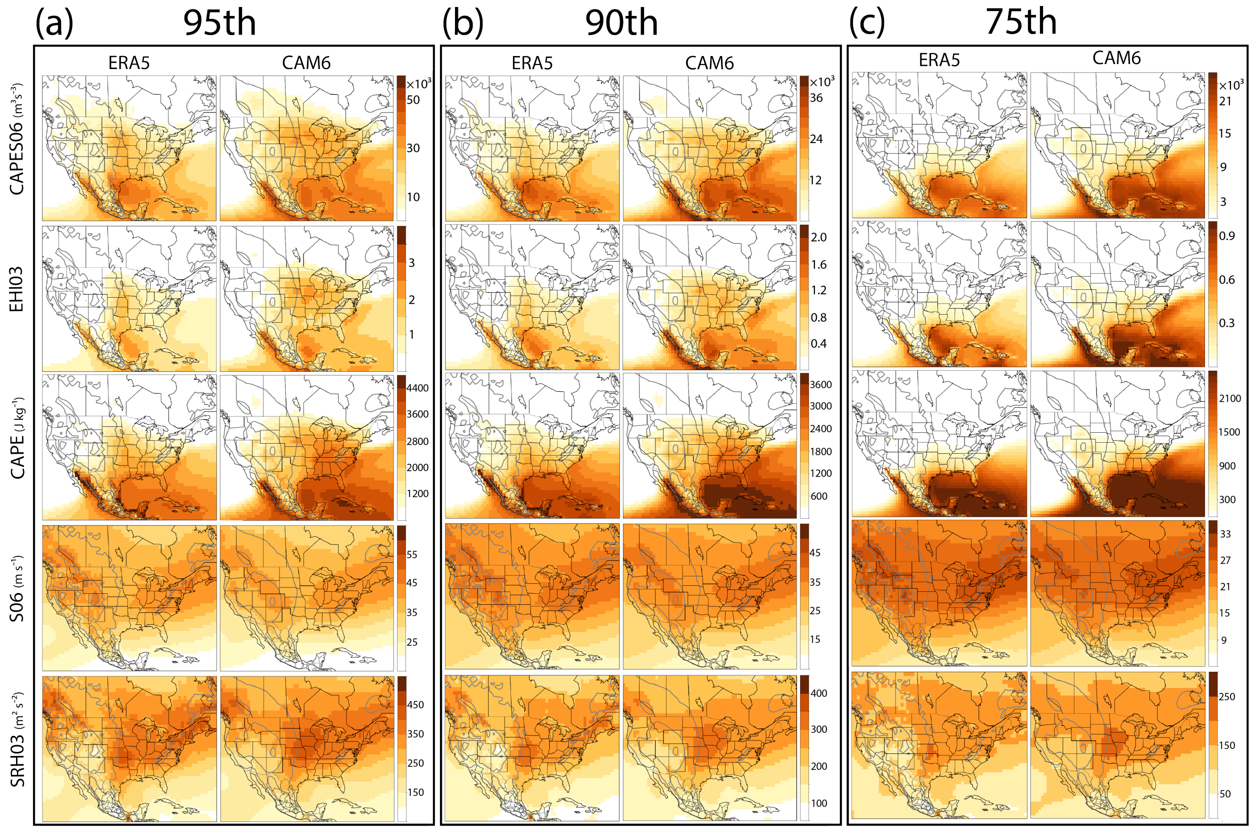


Fig. S4: As in Fig. 4, but for (a) 95th, (b) 90th, and (c) 75th percentiles of CAPES06, EHI03, CAPE, S06, and SRH03 in ERA5 and CAM6.

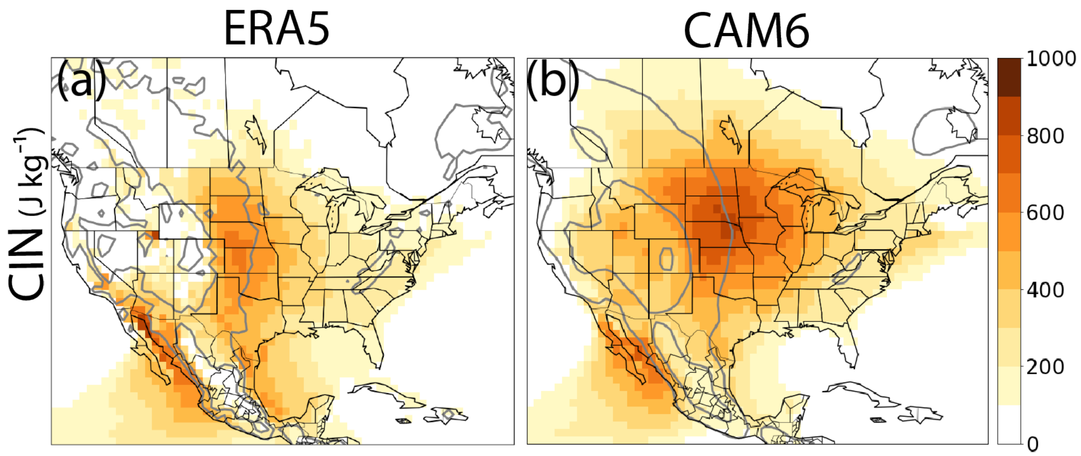


FIG. S5: As in Fig. 4, but for the 99th percentile of CIN (defined as the negative integral of buoyancy from surface to the level of free convection) from (a) ERA5 and (b) CAM6.

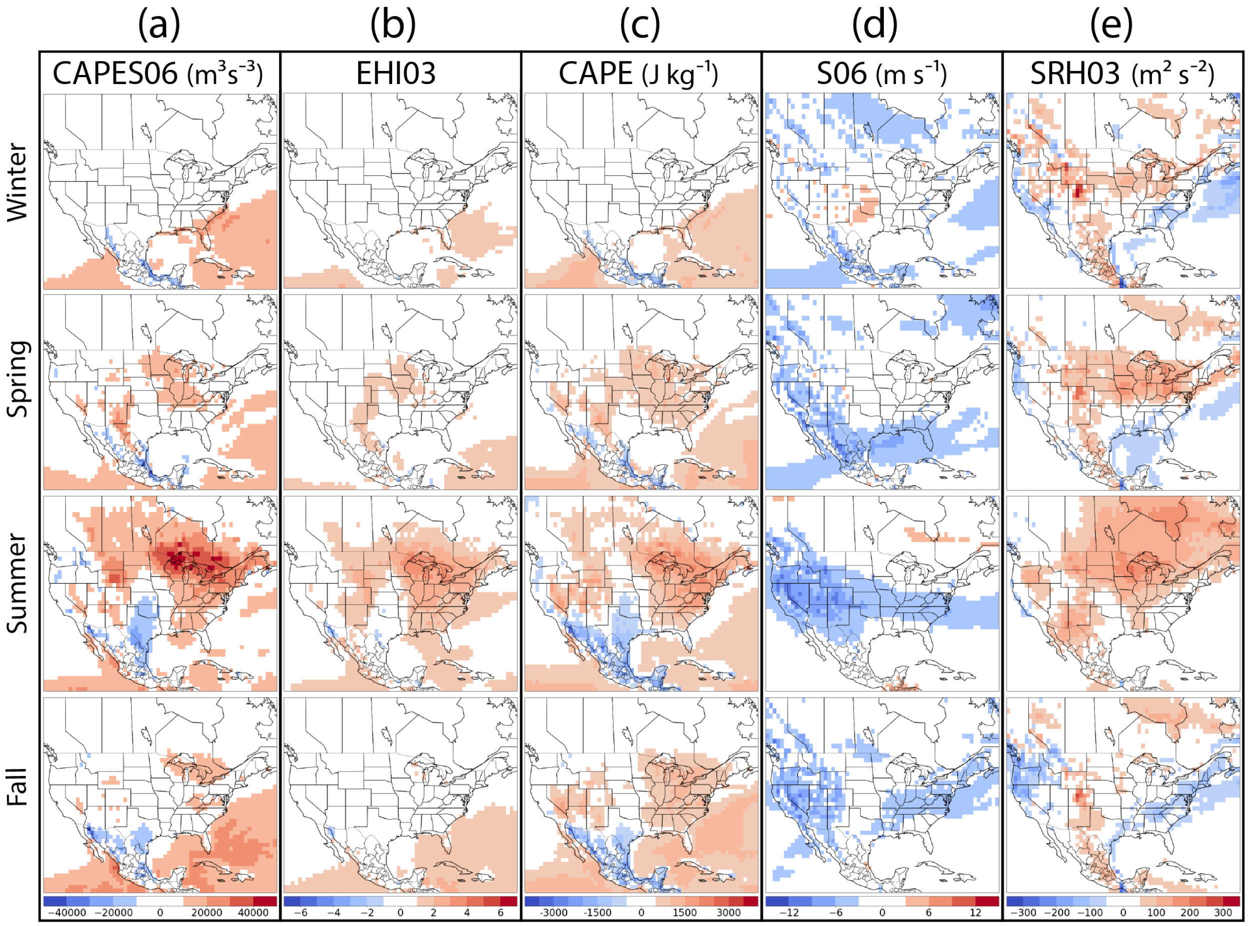


FIG. S6: As in Fig. 5–6, but for the difference (CAM6 minus ERA5).

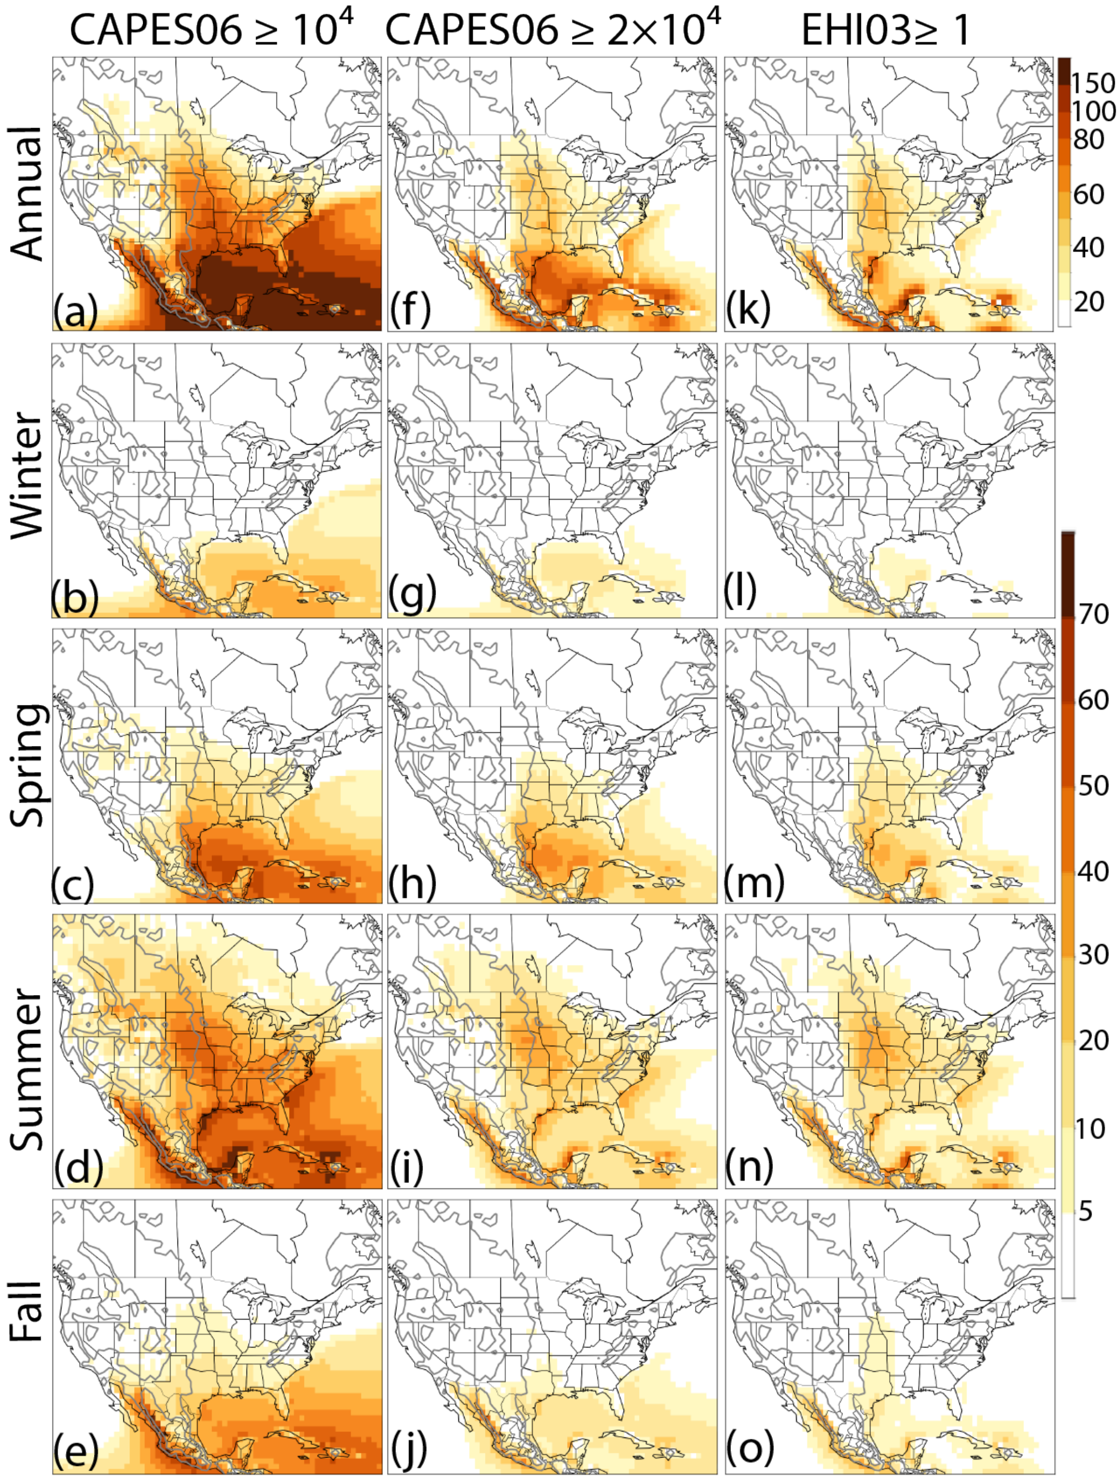


FIG. S7: Mean number of days associated with severe weather environments (NDSEV) from ERA5 reanalysis data during 1980–2014. For CAPES06 $\geq 10^4$ m$^3$ s$^{-3}$: (a) annually, (b) winter (DJF), (c) spring (MAM), (d) summer (JJA), and (e) fall (SON). (f-j) as in (a-e) but for CAPES06 $\geq 2\times10^4$ m$^3$ s$^{-3}$. (k-o) as in (a-e) but for EHI03 $\geq 1$. Grey contour lines denote elevations at 500, 1500, and 2500 m.

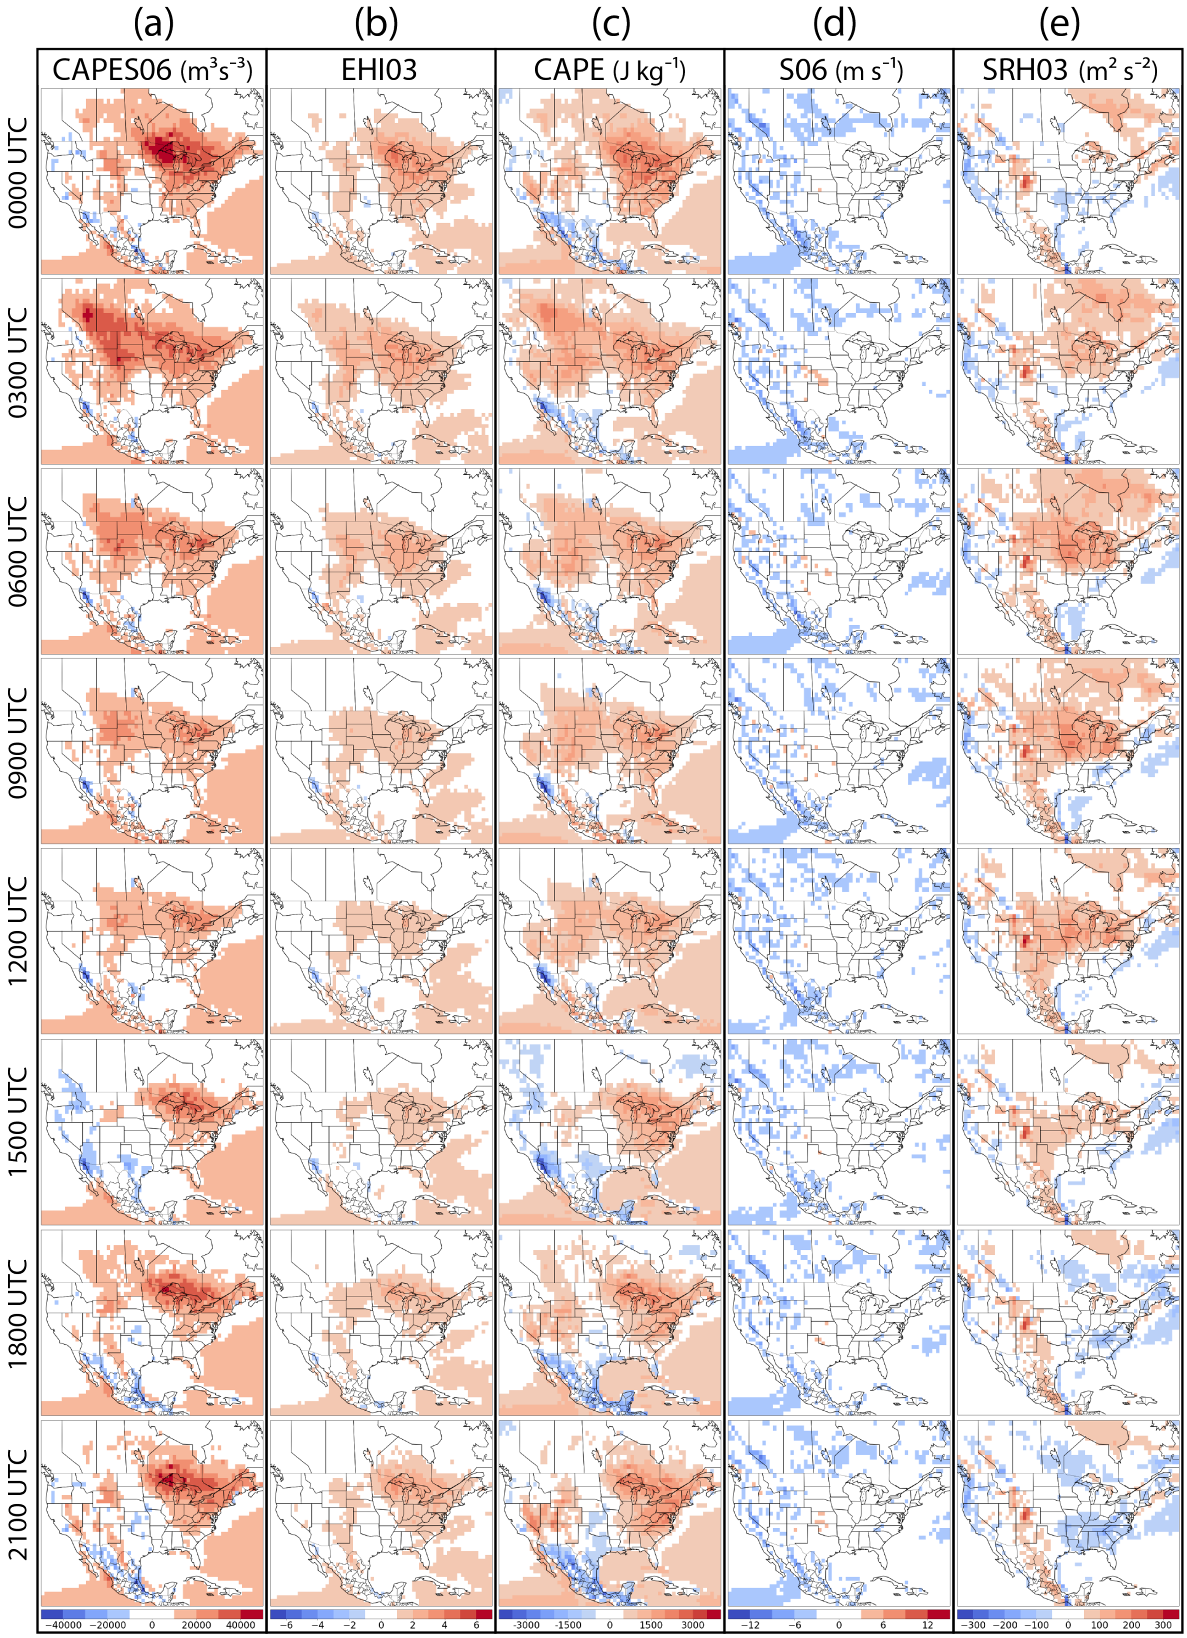


FIG. S8: As in Fig. 7–8, but for the difference (CAM6 minus ERA5).

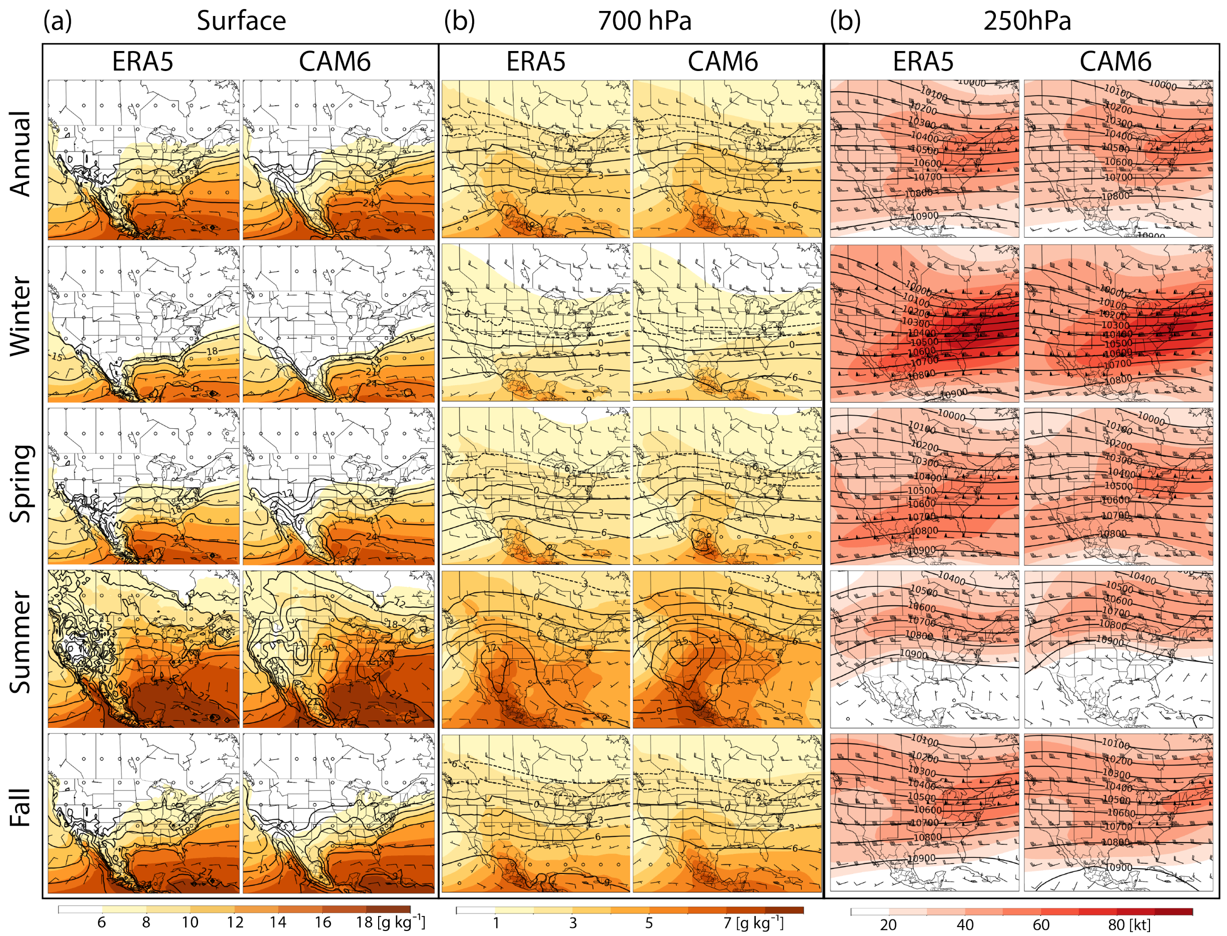


FIG. S9: ERA5 reanalysis vs. CAM6 simulation for the annual and seasonal mean state of atmosphere during 1980–2014. (a) for 10-m wind vector, 2-m air temperature (°C; black contour lines), and 2-m specific humidity (g kg$^{-1}$; filled contours); (b) for 700-hPa wind vector, air temperature (°C; black contour lines), and specific humidity (g kg$^{-1}$; filled contours); (c) for 250-hPa wind vector, geopotential height (m; black contour lines), and wind speed (kts; filled contours).

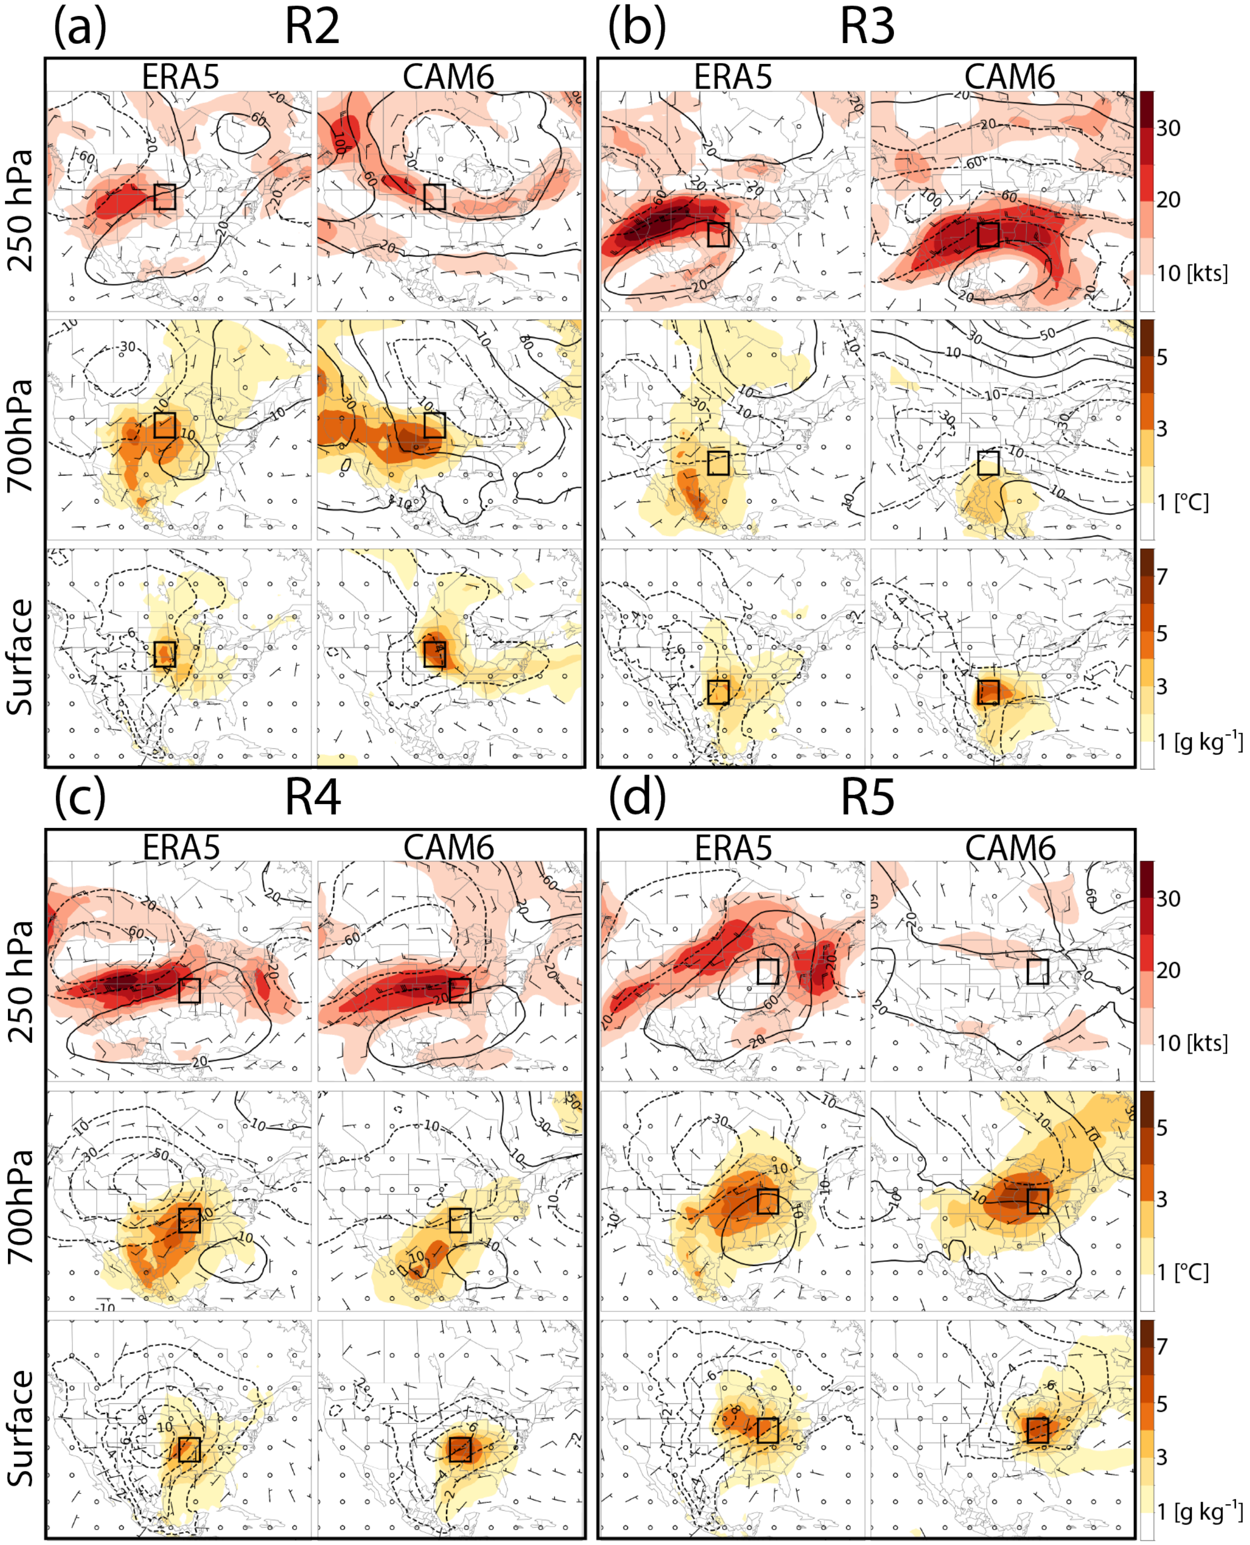


FIG. S10: As in Fig. 15, but for sub-regions of (a) R2, (b) R3, (c) R4, and (d) R5.
